# Supplementary material for: Quantified limits of the nuclear landscape
Source: arXiv:2001.05924 ancillary file (2020-03-31)
Supplement: Supplementary file 1 [file nuclear_landscape_supp.pdf]

# Supplemental Material for "Quantified limits of the nuclear landscape"

Léo Neufcourt,[1,2] Yuchen Cao (曹宇晨),[2,3] Samuel A. Giuliani,[2,3]
Witold Nazarewicz,[2,4] Erik Olsen,[5] and Oleg B. Tarasov[3]

[1] *Department of Statistics and Probability, Michigan State University, East Lansing, Michigan 48824, USA*
[2] *Facility for Rare Isotope Beams, Michigan State University, East Lansing, Michigan 48824, USA*
[3] *National Superconducting Cyclotron Laboratory, Michigan State University, East Lansing, Michigan 48824, USA*
[4] *Department of Physics and Astronomy, Michigan State University, East Lansing, Michigan 48824, USA*
[5] *Institut d'Astronomie et d'Astrophysique, Université Libre de Bruxelles, 1050 Brussels, Belgium*

(Dated: March 9, 2020)

This supplemental material contains additional figures and tables: downloadable pdf versions of Figs. 1 and 2, and a table of posterior predictions of the separation energies of nuclei at the one- and two-particle drip lines.

## I. SUPPLEMENTAL FIGURES

- High-resolution version of Fig. 1: URL
- High-resolution version of Fig. 2: URL

## II. SUPPLEMENTAL TABLES

Table of posterior mean and standard deviation predicted in BMA($n$+$p$) for the nuclear separation energies $S_{1n}$ (odd-$N$ nuclei), $S_{2n}$ (even-$N$ nuclei), $S_{1p}$ (odd-$Z$ nuclei), and $S_{2p}$ (even-$Z$ nuclei) of threshold systems ($0.1 < p_{ex} < 0.9$) [30]. Recall that BMA($n+p$) corresponds to BMA($n$) for neutron-rich nuclei and BMA($p$) for proton-rich nuclei. We provide this table for a rough orientation only as, due to large uncertainties, the quantified predictions are close to zero.

## Posterior predictions of nuclear separation energies (in MeV)

**$S_{1n}$ (odd N)**

| Z | N | $S_{1n}$ | $\sigma_{S_{1n}}$ |
|---|---|---|---|
| 5 | 11 | 0.264 | 0.397 |
| 9 | 19 | -0.150 | 0.361 |
| 13 | 29 | -0.067 | 0.459 |
| 13 | 31 | -0.279 | 0.466 |
| 14 | 31 | -0.038 | 0.499 |
| 15 | 33 | 0.008 | 0.466 |
| 16 | 33 | 0.122 | 0.498 |
| 17 | 35 | 0.056 | 0.459 |
| 18 | 35 | 0.169 | 0.439 |
| 18 | 37 | 0.129 | 0.449 |
| 19 | 39 | 0.259 | 0.467 |
| 20 | 41 | -0.176 | 0.502 |
| 21 | 45 | 0.226 | 0.469 |
| 21 | 47 | -0.079 | 0.469 |
| 22 | 47 | 0.153 | 0.501 |
| 22 | 49 | -0.236 | 0.501 |
| 23 | 51 | 0.040 | 0.467 |
| 23 | 53 | -0.279 | 0.467 |
| 23 | 55 | -0.404 | 0.468 |
| 24 | 51 | 0.037 | 0.501 |
| 24 | 53 | -0.331 | 0.499 |
| 25 | 53 | 0.381 | 0.467 |
| 25 | 55 | 0.198 | 0.470 |
| 25 | 57 | -0.149 | 0.469 |
| 26 | 53 | 0.447 | 0.501 |
| 26 | 55 | 0.117 | 0.502 |
| 26 | 57 | -0.168 | 0.500 |
| 27 | 57 | 0.368 | 0.467 |
| 27 | 59 | -0.195 | 0.468 |
| 28 | 57 | 0.280 | 0.502 |
| 28 | 59 | -0.344 | 0.501 |
| 29 | 59 | 0.275 | 0.469 |
| 29 | 61 | -0.057 | 0.469 |
| 30 | 59 | 0.307 | 0.500 |
| 30 | 61 | 0.022 | 0.499 |
| 30 | 63 | -0.230 | 0.499 |
| 31 | 65 | 0.229 | 0.467 |
| 31 | 67 | 0.056 | 0.469 |
| 31 | 69 | -0.233 | 0.468 |
| 32 | 65 | 0.324 | 0.502 |
| 32 | 67 | 0.091 | 0.500 |
| 32 | 69 | -0.151 | 0.501 |
| 32 | 71 | -0.309 | 0.501 |
| 33 | 71 | 0.323 | 0.468 |
| 33 | 73 | 0.038 | 0.468 |
| 33 | 75 | -0.053 | 0.467 |
| 33 | 77 | -0.271 | 0.468 |
| 34 | 71 | 0.303 | 0.500 |
| 34 | 73 | 0.213 | 0.501 |
| 34 | 75 | -0.066 | 0.500 |
| 34 | 77 | -0.279 | 0.501 |
| 35 | 79 | 0.212 | 0.468 |
| 35 | 81 | -0.145 | 0.469 |
| 36 | 79 | 0.270 | 0.502 |
| 36 | 81 | -0.063 | 0.500 |
| 39 | 83 | 0.088 | 0.467 |
| 39 | 85 | -0.178 | 0.469 |
| 39 | 87 | -0.214 | 0.467 |
| 39 | 89 | -0.348 | 0.468 |
| 40 | 83 | 0.046 | 0.500 |
| 40 | 85 | -0.268 | 0.500 |
| 40 | 87 | -0.327 | 0.500 |
| 41 | 85 | 0.304 | 0.468 |
| 41 | 87 | 0.203 | 0.467 |
| 41 | 89 | 0.087 | 0.468 |
| 41 | 91 | -0.110 | 0.469 |
| 41 | 93 | -0.219 | 0.470 |
| 42 | 83 | 0.473 | 0.500 |
| 42 | 85 | 0.206 | 0.502 |
| 42 | 87 | 0.151 | 0.501 |
| 42 | 89 | -0.063 | 0.500 |

| Z | N | $S_{1n}$ | $\sigma_{S_{1n}}$ |
|---|---|---|---|
| 42 | 91 | -0.251 | 0.501 |
| 43 | 89 | 0.436 | 0.469 |
| 43 | 91 | 0.296 | 0.468 |
| 43 | 93 | 0.015 | 0.469 |
| 43 | 95 | -0.314 | 0.468 |
| 44 | 89 | 0.277 | 0.501 |
| 44 | 91 | 0.109 | 0.501 |
| 44 | 93 | -0.188 | 0.502 |
| 45 | 93 | 0.377 | 0.469 |
| 45 | 95 | 0.015 | 0.468 |
| 45 | 97 | -0.084 | 0.469 |
| 45 | 99 | -0.180 | 0.467 |
| 46 | 93 | 0.156 | 0.501 |
| 46 | 95 | -0.003 | 0.499 |
| 46 | 97 | -0.178 | 0.501 |
| 46 | 99 | -0.248 | 0.500 |
| 47 | 97 | 0.327 | 0.469 |
| 47 | 99 | 0.253 | 0.469 |
| 47 | 101 | 0.061 | 0.467 |
| 47 | 103 | -0.068 | 0.467 |
| 47 | 105 | -0.155 | 0.467 |
| 47 | 107 | -0.284 | 0.468 |
| 48 | 95 | 0.357 | 0.500 |
| 48 | 97 | 0.218 | 0.499 |
| 48 | 99 | 0.245 | 0.500 |
| 48 | 101 | 0.066 | 0.499 |
| 48 | 103 | -0.137 | 0.500 |
| 48 | 105 | -0.237 | 0.501 |
| 48 | 107 | -0.328 | 0.501 |
| 49 | 103 | 0.349 | 0.468 |
| 49 | 105 | 0.280 | 0.468 |
| 49 | 107 | 0.046 | 0.468 |
| 49 | 109 | 0.093 | 0.467 |
| 49 | 111 | -0.172 | 0.469 |
| 49 | 113 | -0.219 | 0.470 |
| 49 | 115 | -0.275 | 0.468 |
| 50 | 103 | 0.332 | 0.500 |
| 50 | 105 | 0.197 | 0.500 |
| 50 | 107 | 0.061 | 0.501 |
| 50 | 109 | -0.086 | 0.501 |
| 50 | 111 | -0.181 | 0.501 |
| 50 | 113 | -0.261 | 0.502 |
| 50 | 115 | -0.302 | 0.499 |
| 50 | 119 | -0.339 | 0.501 |
| 51 | 111 | 0.342 | 0.467 |
| 51 | 113 | 0.230 | 0.468 |
| 51 | 115 | 0.169 | 0.467 |
| 51 | 117 | 0.076 | 0.467 |
| 51 | 119 | 0.141 | 0.467 |
| 51 | 121 | 0.100 | 0.466 |
| 51 | 123 | 0.062 | 0.488 |
| 52 | 111 | 0.178 | 0.501 |
| 52 | 113 | 0.026 | 0.502 |
| 52 | 115 | 0.048 | 0.500 |
| 52 | 117 | 0.042 | 0.502 |
| 52 | 119 | -0.043 | 0.501 |
| 52 | 121 | -0.003 | 0.501 |
| 52 | 123 | -0.010 | 0.501 |
| 53 | 123 | 0.431 | 0.468 |
| 53 | 125 | -0.020 | 0.469 |
| 54 | 115 | 0.387 | 0.499 |
| 54 | 117 | 0.350 | 0.500 |
| 54 | 119 | 0.337 | 0.500 |
| 54 | 121 | 0.350 | 0.500 |
| 54 | 123 | 0.392 | 0.502 |
| 54 | 125 | -0.085 | 0.503 |
| 61 | 127 | -0.208 | 0.468 |
| 61 | 129 | -0.209 | 0.468 |
| 61 | 131 | -0.064 | 0.468 |
| 61 | 133 | -0.199 | 0.468 |
| 61 | 137 | -0.171 | 0.466 |
| 61 | 139 | -0.191 | 0.467 |
| 61 | 141 | -0.322 | 0.474 |
| 62 | 127 | -0.170 | 0.502 |
| 62 | 129 | -0.363 | 0.500 |
| 62 | 131 | -0.244 | 0.501 |

| Z | N | $S_{1n}$ | $\sigma_{S_{1n}}$ |
|---|---|---|---|
| 62 | 137 | -0.220 | 0.500 |
| 62 | 139 | -0.293 | 0.500 |
| 63 | 127 | 0.315 | 0.466 |
| 63 | 129 | 0.136 | 0.468 |
| 63 | 131 | 0.220 | 0.469 |
| 63 | 133 | 0.086 | 0.467 |
| 63 | 135 | 0.116 | 0.469 |
| 63 | 137 | 0.260 | 0.467 |
| 63 | 139 | 0.212 | 0.467 |
| 63 | 141 | 0.163 | 0.469 |
| 63 | 143 | -0.021 | 0.468 |
| 63 | 145 | -0.256 | 0.468 |
| 64 | 127 | 0.215 | 0.501 |
| 64 | 129 | 0.024 | 0.501 |
| 64 | 131 | 0.099 | 0.500 |
| 64 | 133 | -0.039 | 0.501 |
| 64 | 135 | -0.036 | 0.502 |
| 64 | 137 | 0.163 | 0.501 |
| 64 | 139 | 0.082 | 0.500 |
| 64 | 141 | 0.070 | 0.501 |
| 64 | 143 | -0.129 | 0.499 |
| 65 | 145 | 0.181 | 0.469 |
| 65 | 147 | -0.034 | 0.469 |
| 65 | 149 | -0.257 | 0.468 |
| 66 | 129 | 0.434 | 0.502 |
| 66 | 143 | 0.261 | 0.500 |
| 66 | 145 | -0.013 | 0.501 |
| 66 | 147 | -0.149 | 0.500 |
| 67 | 147 | 0.261 | 0.469 |
| 67 | 149 | 0.123 | 0.467 |
| 67 | 151 | 0.029 | 0.466 |
| 67 | 153 | -0.202 | 0.466 |
| 68 | 147 | 0.216 | 0.500 |
| 68 | 149 | 0.019 | 0.501 |
| 68 | 151 | -0.110 | 0.500 |
| 68 | 153 | -0.252 | 0.501 |
| 69 | 153 | 0.201 | 0.468 |
| 69 | 155 | 0.148 | 0.468 |
| 69 | 157 | -0.115 | 0.468 |
| 70 | 151 | 0.246 | 0.500 |
| 70 | 153 | 0.142 | 0.499 |
| 70 | 155 | 0.024 | 0.500 |
| 70 | 157 | -0.255 | 0.501 |
| 71 | 157 | 0.223 | 0.468 |
| 71 | 159 | -0.003 | 0.467 |
| 71 | 161 | -0.151 | 0.467 |
| 72 | 155 | 0.302 | 0.502 |
| 72 | 157 | 0.124 | 0.500 |
| 72 | 159 | -0.102 | 0.501 |
| 72 | 161 | -0.311 | 0.500 |
| 73 | 159 | 0.321 | 0.468 |
| 73 | 161 | 0.240 | 0.467 |
| 73 | 163 | 0.065 | 0.468 |
| 73 | 165 | -0.078 | 0.468 |
| 73 | 167 | -0.145 | 0.469 |
| 73 | 169 | -0.283 | 0.467 |
| 73 | 171 | -0.225 | 0.489 |
| 73 | 173 | -0.286 | 0.488 |
| 73 | 175 | -0.299 | 0.488 |
| 73 | 181 | -0.139 | 0.496 |
| 74 | 159 | 0.202 | 0.501 |
| 74 | 161 | 0.097 | 0.499 |
| 74 | 163 | -0.026 | 0.502 |
| 74 | 165 | -0.122 | 0.502 |
| 74 | 167 | -0.234 | 0.502 |
| 74 | 169 | -0.303 | 0.501 |
| 74 | 181 | -0.278 | 0.532 |
| 75 | 165 | 0.354 | 0.469 |
| 75 | 167 | 0.221 | 0.469 |
| 75 | 169 | 0.115 | 0.468 |
| 75 | 171 | 0.082 | 0.467 |
| 75 | 173 | -0.023 | 0.468 |
| 75 | 175 | -0.049 | 0.469 |
| 75 | 177 | -0.011 | 0.488 |
| 75 | 179 | -0.055 | 0.497 |
| 75 | 181 | 0.208 | 0.497 |

| Z | N | $S_{1n}$ | $\sigma_{S_{1n}}$ |
|---|---|---|---|
| 75 | 183 | -0.176 | 0.496 |
| 76 | 163 | 0.363 | 0.501 |
| 76 | 165 | 0.246 | 0.501 |
| 76 | 167 | 0.178 | 0.502 |
| 76 | 169 | 0.042 | 0.500 |
| 76 | 171 | 0.024 | 0.501 |
| 76 | 173 | -0.073 | 0.501 |
| 76 | 175 | -0.217 | 0.501 |
| 76 | 177 | -0.184 | 0.500 |
| 76 | 179 | -0.180 | 0.519 |
| 76 | 181 | 0.089 | 0.520 |
| 76 | 183 | -0.340 | 0.521 |
| 77 | 175 | 0.374 | 0.467 |
| 77 | 177 | 0.302 | 0.468 |
| 77 | 179 | 0.195 | 0.467 |
| 77 | 183 | 0.120 | 0.486 |
| 78 | 173 | 0.397 | 0.500 |
| 78 | 175 | 0.289 | 0.502 |
| 78 | 177 | 0.195 | 0.502 |
| 78 | 179 | 0.110 | 0.502 |
| 78 | 181 | 0.310 | 0.500 |
| 78 | 183 | -0.039 | 0.521 |
| 79 | 183 | 0.337 | 0.468 |
| 80 | 183 | 0.183 | 0.501 |
| 87 | 185 | -0.145 | 0.468 |
| 87 | 191 | -0.322 | 0.468 |
| 87 | 197 | -0.258 | 0.468 |
| 88 | 197 | -0.290 | 0.502 |
| 89 | 185 | 0.078 | 0.468 |
| 89 | 187 | -0.164 | 0.468 |
| 89 | 189 | -0.037 | 0.467 |
| 89 | 191 | -0.071 | 0.467 |
| 89 | 193 | -0.025 | 0.467 |
| 89 | 195 | 0.153 | 0.468 |
| 89 | 197 | 0.203 | 0.468 |
| 89 | 199 | 0.146 | 0.468 |
| 89 | 201 | -0.034 | 0.474 |
| 89 | 203 | -0.173 | 0.473 |
| 90 | 185 | -0.078 | 0.501 |
| 90 | 187 | -0.307 | 0.502 |
| 90 | 189 | -0.191 | 0.502 |
| 90 | 191 | -0.241 | 0.499 |
| 90 | 193 | -0.111 | 0.502 |
| 90 | 195 | 0.111 | 0.501 |
| 90 | 197 | 0.107 | 0.500 |
| 90 | 199 | 0.020 | 0.500 |
| 90 | 201 | -0.024 | 0.501 |
| 90 | 203 | -0.249 | 0.498 |
| 91 | 185 | 0.358 | 0.467 |
| 91 | 187 | 0.150 | 0.467 |
| 91 | 189 | 0.254 | 0.467 |
| 91 | 191 | 0.206 | 0.469 |
| 91 | 193 | 0.262 | 0.466 |
| 91 | 201 | 0.396 | 0.468 |
| 91 | 203 | 0.314 | 0.468 |
| 91 | 205 | 0.063 | 0.468 |
| 91 | 207 | -0.089 | 0.468 |
| 91 | 209 | -0.255 | 0.467 |
| 91 | 211 | -0.280 | 0.468 |
| 91 | 213 | -0.287 | 0.489 |
| 92 | 185 | 0.201 | 0.501 |
| 92 | 187 | 0.006 | 0.501 |
| 92 | 189 | 0.081 | 0.501 |
| 92 | 191 | 0.050 | 0.501 |
| 92 | 193 | 0.254 | 0.501 |
| 92 | 195 | 0.479 | 0.501 |
| 92 | 197 | 0.441 | 0.501 |
| 92 | 199 | 0.435 | 0.502 |
| 92 | 201 | 0.351 | 0.501 |
| 92 | 203 | 0.148 | 0.500 |
| 92 | 205 | -0.028 | 0.500 |
| 92 | 207 | -0.219 | 0.501 |
| 92 | 209 | -0.357 | 0.500 |
| 93 | 207 | 0.255 | 0.469 |
| 93 | 209 | 0.092 | 0.467 |
| 93 | 211 | -0.061 | 0.468 |

| Z | N | $S_{1n}$ | $\sigma_{S_{1n}}$ |
|---|---|---|---|
| 93 | 213 | -0.193 | 0.468 |
| 93 | 215 | -0.310 | 0.467 |
| 94 | 187 | 0.331 | 0.500 |
| 94 | 189 | 0.389 | 0.501 |
| 94 | 191 | 0.458 | 0.501 |
| 94 | 205 | 0.294 | 0.501 |
| 94 | 207 | 0.123 | 0.501 |
| 94 | 209 | -0.024 | 0.500 |
| 94 | 211 | -0.200 | 0.501 |
| 94 | 213 | -0.315 | 0.500 |
| 95 | 209 | 0.360 | 0.467 |
| 95 | 211 | 0.203 | 0.466 |
| 95 | 213 | 0.069 | 0.467 |
| 95 | 215 | -0.101 | 0.468 |
| 95 | 217 | -0.246 | 0.468 |
| 95 | 219 | -0.329 | 0.468 |
| 96 | 209 | 0.235 | 0.500 |
| 96 | 211 | 0.085 | 0.499 |
| 96 | 213 | -0.029 | 0.502 |
| 96 | 215 | -0.184 | 0.503 |
| 96 | 217 | -0.312 | 0.502 |
| 97 | 213 | 0.391 | 0.467 |
| 97 | 215 | 0.230 | 0.469 |
| 97 | 217 | 0.092 | 0.468 |
| 97 | 219 | -0.110 | 0.467 |
| 97 | 221 | -0.199 | 0.469 |
| 97 | 223 | -0.281 | 0.468 |
| 98 | 211 | 0.435 | 0.501 |
| 98 | 213 | 0.280 | 0.500 |
| 98 | 215 | 0.075 | 0.500 |
| 98 | 217 | -0.055 | 0.500 |
| 98 | 219 | -0.188 | 0.501 |
| 99 | 219 | 0.227 | 0.467 |
| 99 | 221 | 0.029 | 0.468 |
| 99 | 223 | -0.086 | 0.470 |
| 99 | 225 | -0.148 | 0.467 |
| 99 | 227 | -0.235 | 0.467 |
| 99 | 255 | -0.393 | 0.496 |
| 100 | 219 | 0.317 | 0.500 |
| 100 | 221 | 0.110 | 0.500 |
| 100 | 223 | 0.054 | 0.501 |
| 100 | 225 | -0.080 | 0.501 |
| 100 | 227 | -0.203 | 0.499 |
| 100 | 229 | -0.264 | 0.500 |
| 101 | 223 | 0.464 | 0.469 |
| 101 | 225 | 0.355 | 0.467 |
| 101 | 227 | 0.193 | 0.467 |
| 101 | 229 | 0.109 | 0.468 |
| 101 | 231 | -0.012 | 0.469 |
| 101 | 233 | -0.148 | 0.467 |
| 101 | 235 | -0.165 | 0.488 |
| 101 | 237 | -0.215 | 0.488 |
| 101 | 239 | -0.150 | 0.488 |
| 101 | 241 | -0.021 | 0.489 |
| 101 | 243 | -0.165 | 0.498 |
| 101 | 245 | -0.246 | 0.497 |
| 101 | 247 | -0.319 | 0.497 |
| 101 | 249 | -0.357 | 0.497 |
| 101 | 255 | -0.146 | 0.497 |
| 102 | 221 | 0.439 | 0.499 |
| 102 | 223 | 0.295 | 0.502 |
| 102 | 225 | 0.215 | 0.501 |
| 102 | 227 | 0.050 | 0.500 |
| 102 | 229 | -0.085 | 0.501 |
| 102 | 231 | -0.217 | 0.500 |
| 102 | 233 | -0.363 | 0.499 |
| 102 | 239 | -0.409 | 0.521 |
| 102 | 241 | -0.317 | 0.521 |
| 102 | 243 | -0.418 | 0.533 |
| 103 | 229 | 0.397 | 0.469 |
| 103 | 231 | 0.221 | 0.469 |
| 103 | 233 | 0.014 | 0.468 |
| 103 | 235 | -0.135 | 0.468 |
| 103 | 237 | -0.020 | 0.487 |
| 103 | 239 | -0.090 | 0.488 |
| 103 | 241 | 0.097 | 0.489 |
| 103 | 243 | 0.051 | 0.488 |
| 103 | 245 | -0.079 | 0.496 |
| 103 | 247 | -0.159 | 0.497 |
| 103 | 249 | -0.213 | 0.498 |

| Z | N | $S_{1n}$ | $\sigma_{S_{1n}}$ |
|---|---|---|---|
| 103 | 251 | -0.269 | 0.498 |
| 103 | 253 | -0.294 | 0.496 |
| 103 | 255 | -0.041 | 0.497 |
| 103 | 257 | -0.389 | 0.496 |
| 104 | 225 | 0.506 | 0.501 |
| 104 | 227 | 0.340 | 0.498 |
| 104 | 229 | 0.232 | 0.501 |
| 104 | 231 | 0.007 | 0.501 |
| 104 | 233 | -0.129 | 0.499 |
| 104 | 235 | -0.263 | 0.502 |
| 104 | 237 | -0.216 | 0.519 |
| 104 | 239 | -0.342 | 0.520 |
| 104 | 241 | -0.157 | 0.519 |
| 104 | 243 | -0.148 | 0.519 |
| 104 | 245 | -0.294 | 0.521 |
| 104 | 247 | -0.419 | 0.532 |
| 104 | 255 | -0.318 | 0.532 |
| 105 | 233 | 0.291 | 0.466 |
| 105 | 235 | 0.169 | 0.488 |
| 105 | 237 | 0.157 | 0.487 |
| 105 | 239 | 0.082 | 0.487 |
| 105 | 241 | 0.126 | 0.488 |
| 105 | 243 | 0.240 | 0.490 |
| 105 | 245 | 0.161 | 0.487 |
| 105 | 247 | 0.064 | 0.487 |
| 105 | 249 | 0.003 | 0.498 |
| 105 | 251 | -0.147 | 0.496 |
| 105 | 253 | -0.179 | 0.497 |
| 105 | 255 | 0.096 | 0.497 |
| 105 | 257 | -0.212 | 0.497 |
| 106 | 231 | 0.316 | 0.501 |
| 106 | 233 | 0.108 | 0.500 |
| 106 | 235 | 0.008 | 0.520 |
| 106 | 237 | -0.077 | 0.520 |
| 106 | 239 | -0.131 | 0.521 |
| 106 | 241 | -0.098 | 0.519 |
| 106 | 243 | 0.021 | 0.519 |
| 106 | 245 | -0.089 | 0.521 |
| 106 | 247 | -0.175 | 0.521 |
| 106 | 249 | -0.101 | 0.521 |
| 106 | 251 | -0.433 | 0.532 |
| 106 | 255 | -0.145 | 0.532 |
| 107 | 189 | 2.652 | 0.468 |
| 107 | 235 | 0.434 | 0.489 |
| 107 | 237 | 0.367 | 0.487 |
| 107 | 239 | 0.352 | 0.488 |
| 107 | 241 | 0.277 | 0.488 |
| 107 | 243 | 0.352 | 0.488 |
| 107 | 245 | 0.367 | 0.488 |
| 107 | 247 | 0.298 | 0.489 |
| 107 | 249 | 0.287 | 0.488 |
| 107 | 251 | 0.130 | 0.488 |
| 107 | 253 | 0.014 | 0.488 |
| 107 | 255 | 0.269 | 0.495 |
| 107 | 257 | -0.062 | 0.498 |
| 108 | 233 | 0.438 | 0.519 |
| 108 | 235 | 0.264 | 0.520 |
| 108 | 237 | 0.154 | 0.521 |
| 108 | 239 | 0.064 | 0.520 |
| 108 | 241 | 0.121 | 0.520 |
| 108 | 243 | 0.046 | 0.520 |
| 108 | 245 | 0.117 | 0.520 |
| 108 | 247 | 0.091 | 0.521 |
| 108 | 249 | -0.027 | 0.521 |
| 108 | 251 | -0.057 | 0.519 |
| 108 | 253 | -0.195 | 0.520 |
| 108 | 255 | 0.059 | 0.531 |
| 108 | 257 | -0.331 | 0.532 |
| 109 | 249 | 0.452 | 0.488 |
| 109 | 251 | 0.304 | 0.498 |
| 109 | 253 | 0.194 | 0.497 |
| 109 | 255 | 0.471 | 0.496 |
| 109 | 257 | 0.102 | 0.497 |
| 110 | 237 | 0.448 | 0.522 |
| 110 | 239 | 0.385 | 0.519 |
| 110 | 241 | 0.333 | 0.520 |
| 110 | 243 | 0.230 | 0.520 |
| 110 | 245 | 0.299 | 0.519 |
| 110 | 247 | 0.322 | 0.521 |
| 110 | 249 | 0.283 | 0.520 |

**$S_{1n}$ (odd N)**

| Z | N | $S_{1n}$ | $\sigma_{S_{1n}}$ |
|---|---|---|---|
| 110 | 251 | 0.078 | 0.534 |
| 110 | 253 | 0.002 | 0.532 |
| 110 | 255 | 0.236 | 0.532 |
| 110 | 257 | -0.112 | 0.531 |
| 111 | 253 | 0.476 | 0.498 |
| 111 | 257 | 0.295 | 0.498 |
| 111 | 273 | -0.145 | 0.495 |
| 112 | 243 | 0.471 | 0.534 |
| 112 | 245 | 0.434 | 0.532 |
| 112 | 247 | 0.471 | 0.531 |
| 112 | 249 | 0.436 | 0.531 |
| 112 | 251 | 0.344 | 0.532 |
| 112 | 253 | 0.309 | 0.531 |
| 112 | 255 | 0.471 | 0.534 |
| 112 | 257 | 0.078 | 0.533 |
| 112 | 273 | -0.215 | 0.532 |
| 113 | 257 | 0.485 | 0.499 |
| 113 | 273 | 0.012 | 0.496 |
| 113 | 275 | -0.153 | 0.495 |
| 113 | 277 | -0.331 | 0.497 |
| 114 | 253 | 0.576 | 0.534 |
| 114 | 257 | 0.274 | 0.533 |
| 114 | 275 | -0.297 | 0.531 |
| 115 | 259 | -0.100 | 0.499 |
| 115 | 269 | -0.251 | 0.496 |
| 115 | 271 | -0.194 | 0.496 |
| 115 | 273 | 0.080 | 0.499 |
| 115 | 275 | -0.026 | 0.496 |
| 115 | 277 | -0.121 | 0.497 |
| 115 | 279 | -0.365 | 0.497 |
| 115 | 281 | -0.420 | 0.498 |
| 115 | 283 | -0.410 | 0.497 |
| 115 | 285 | -0.407 | 0.497 |
| 116 | 257 | 0.486 | 0.532 |
| 116 | 259 | -0.277 | 0.531 |
| 116 | 273 | -0.086 | 0.532 |
| 116 | 277 | -0.360 | 0.531 |
| 117 | 259 | 0.163 | 0.497 |
| 117 | 261 | -0.249 | 0.498 |
| 117 | 263 | -0.302 | 0.495 |
| 117 | 265 | -0.275 | 0.498 |
| 117 | 267 | -0.168 | 0.496 |
| 117 | 269 | -0.080 | 0.496 |
| 117 | 271 | 0.063 | 0.496 |
| 117 | 273 | 0.263 | 0.497 |
| 117 | 275 | -0.013 | 0.497 |
| 117 | 277 | -0.001 | 0.498 |
| 117 | 279 | -0.129 | 0.497 |
| 117 | 281 | -0.251 | 0.497 |
| 117 | 283 | -0.258 | 0.497 |
| 117 | 285 | -0.281 | 0.497 |
| 117 | 287 | -0.342 | 0.496 |
| 117 | 289 | -0.389 | 0.497 |
| 118 | 259 | -0.021 | 0.530 |
| 118 | 269 | -0.325 | 0.532 |
| 118 | 271 | -0.105 | 0.533 |
| 118 | 273 | -0.069 | 0.531 |
| 118 | 275 | -0.276 | 0.532 |
| 118 | 277 | -0.297 | 0.532 |
| 118 | 279 | -0.241 | 0.534 |
| 119 | 259 | 0.412 | 0.495 |
| 119 | 261 | 0.018 | 0.498 |
| 119 | 263 | -0.043 | 0.497 |
| 119 | 265 | -0.036 | 0.498 |
| 119 | 267 | 0.067 | 0.497 |
| 119 | 269 | 0.102 | 0.496 |
| 119 | 271 | 0.242 | 0.496 |
| 119 | 273 | 0.345 | 0.496 |
| 119 | 275 | 0.222 | 0.496 |
| 119 | 277 | 0.199 | 0.499 |
| 119 | 279 | 0.135 | 0.497 |
| 119 | 281 | -0.083 | 0.497 |
| 119 | 283 | -0.124 | 0.496 |
| 119 | 285 | -0.138 | 0.497 |
| 119 | 287 | -0.209 | 0.498 |
| 119 | 289 | -0.246 | 0.498 |
| 119 | 291 | -0.289 | 0.497 |
| 119 | 293 | -0.363 | 0.498 |

**$S_{2n}$ (even N)**

| Z | N | $S_{2n}$ | $\sigma_{S_{2n}}$ |
|---|---|---|---|
| 8 | 20 | -0.170 | 0.835 |
| 9 | 22 | -0.104 | 0.496 |
| 10 | 26 | -0.609 | 0.868 |
| 11 | 28 | 0.297 | 0.696 |
| 11 | 30 | -0.783 | 0.718 |
| 11 | 32 | -0.887 | 0.718 |
| 12 | 30 | 0.332 | 0.869 |
| 12 | 32 | 0.003 | 0.870 |
| 13 | 34 | -0.041 | 0.721 |
| 14 | 34 | 0.721 | 0.872 |
| 16 | 36 | 0.191 | 0.872 |
| 16 | 38 | -0.642 | 0.873 |
| 17 | 40 | -0.015 | 0.720 |
| 18 | 42 | -0.089 | 0.870 |
| 19 | 44 | 0.513 | 0.722 |
| 19 | 46 | -0.001 | 0.721 |
| 19 | 48 | 0.076 | 0.720 |
| 19 | 50 | -0.461 | 0.752 |
| 20 | 48 | 0.706 | 0.871 |
| 20 | 50 | 0.194 | 0.872 |
| 20 | 52 | -0.392 | 0.923 |
| 20 | 54 | -0.752 | 0.920 |
| 20 | 56 | -0.924 | 0.919 |
| 21 | 52 | 0.232 | 0.721 |
| 21 | 54 | -0.236 | 0.721 |
| 21 | 56 | -0.429 | 0.719 |
| 21 | 58 | -0.914 | 0.719 |
| 22 | 52 | 0.780 | 0.870 |
| 22 | 54 | 0.210 | 0.871 |
| 22 | 56 | 0.043 | 0.870 |
| 22 | 58 | -0.570 | 0.871 |
| 23 | 56 | 0.518 | 0.721 |
| 23 | 58 | -0.070 | 0.719 |
| 23 | 60 | -0.870 | 0.717 |
| 24 | 56 | 0.953 | 0.871 |
| 24 | 58 | 0.424 | 0.868 |
| 24 | 60 | -0.562 | 0.868 |
| 25 | 58 | 1.002 | 0.720 |
| 25 | 60 | -0.036 | 0.721 |
| 26 | 60 | 0.429 | 0.871 |
| 26 | 62 | -0.469 | 0.870 |
| 27 | 62 | 0.121 | 0.719 |
| 28 | 64 | -0.009 | 0.872 |
| 28 | 68 | -0.624 | 0.923 |
| 29 | 66 | 0.347 | 0.721 |
| 29 | 68 | 0.235 | 0.720 |
| 29 | 70 | -0.237 | 0.721 |
| 30 | 70 | 0.490 | 0.870 |
| 30 | 72 | 0.007 | 0.872 |
| 30 | 74 | -0.321 | 0.869 |
| 30 | 76 | -0.604 | 0.870 |
| 31 | 74 | 0.447 | 0.721 |
| 31 | 76 | 0.067 | 0.721 |
| 31 | 78 | -0.336 | 0.750 |
| 32 | 76 | 0.647 | 0.867 |
| 32 | 78 | 0.191 | 0.869 |
| 32 | 80 | -0.304 | 0.922 |
| 33 | 80 | 0.332 | 0.719 |
| 33 | 82 | -0.144 | 0.722 |
| 34 | 82 | 0.385 | 0.867 |
| 34 | 84 | -0.658 | 0.869 |
| 35 | 84 | -0.292 | 0.719 |
| 35 | 86 | -0.712 | 0.719 |
| 36 | 84 | 0.056 | 0.872 |
| 36 | 86 | -0.355 | 0.869 |
| 36 | 88 | -0.608 | 0.870 |
| 36 | 90 | -0.696 | 0.924 |
| 37 | 84 | 0.507 | 0.719 |
| 37 | 86 | -0.012 | 0.720 |
| 37 | 88 | -0.211 | 0.719 |
| 37 | 90 | -0.558 | 0.719 |
| 37 | 92 | -0.520 | 0.807 |
| 37 | 94 | -0.760 | 0.805 |
| 38 | 84 | 0.893 | 0.870 |
| 38 | 86 | 0.198 | 0.869 |
| 38 | 88 | 0.075 | 0.870 |
| 38 | 90 | -0.204 | 0.870 |
| 38 | 92 | -0.434 | 0.871 |
| 38 | 94 | -0.278 | 0.998 |
| 39 | 86 | 0.690 | 0.721 |
| 39 | 88 | 0.565 | 0.717 |
| 39 | 90 | 0.286 | 0.718 |
| 39 | 92 | 0.043 | 0.721 |
| 39 | 94 | -0.084 | 0.750 |
| 39 | 96 | -0.664 | 0.809 |
| 40 | 88 | 0.947 | 0.869 |
| 40 | 90 | 0.700 | 0.870 |
| 40 | 92 | 0.421 | 0.869 |
| 40 | 94 | 0.130 | 0.869 |
| 40 | 96 | -0.548 | 0.922 |
| 41 | 92 | 0.867 | 0.720 |
| 41 | 94 | 0.473 | 0.720 |
| 41 | 96 | -0.214 | 0.751 |
| 42 | 94 | 0.749 | 0.869 |
| 42 | 96 | 0.052 | 0.868 |
| 42 | 98 | -0.502 | 0.869 |
| 43 | 96 | 0.424 | 0.719 |
| 43 | 98 | 0.020 | 0.719 |
| 43 | 100 | -0.224 | 0.719 |
| 43 | 102 | -0.398 | 0.717 |
| 44 | 98 | 0.477 | 0.872 |
| 44 | 100 | 0.219 | 0.871 |
| 44 | 102 | 0.104 | 0.867 |
| 44 | 104 | -0.246 | 0.870 |
| 44 | 106 | -0.511 | 0.868 |
| 44 | 108 | -0.554 | 0.992 |
| 45 | 102 | 0.555 | 0.719 |
| 45 | 104 | 0.316 | 0.721 |
| 45 | 106 | 0.062 | 0.719 |
| 45 | 108 | -0.131 | 0.751 |
| 45 | 110 | -0.249 | 0.807 |
| 45 | 112 | -0.519 | 0.808 |
| 46 | 106 | 0.500 | 0.870 |
| 46 | 108 | 0.271 | 0.869 |
| 46 | 110 | 0.027 | 0.923 |
| 46 | 112 | -0.134 | 0.995 |
| 46 | 114 | -0.381 | 0.994 |
| 46 | 116 | -0.658 | 0.996 |
| 47 | 110 | 0.542 | 0.750 |
| 47 | 112 | 0.278 | 0.749 |
| 47 | 114 | 0.173 | 0.806 |
| 47 | 116 | -0.073 | 0.808 |
| 47 | 118 | -0.261 | 0.806 |
| 47 | 120 | -0.388 | 0.805 |
| 48 | 112 | 0.642 | 0.870 |
| 48 | 114 | 0.392 | 0.872 |
| 48 | 116 | 0.386 | 0.995 |
| 48 | 118 | 0.216 | 0.994 |
| 48 | 120 | 0.027 | 0.993 |
| 48 | 122 | -0.130 | 0.994 |
| 48 | 124 | -0.186 | 0.992 |
| 49 | 122 | 0.585 | 0.807 |
| 49 | 124 | 0.429 | 0.807 |
| 49 | 126 | -0.508 | 0.806 |
| 50 | 126 | -0.114 | 0.923 |
| 51 | 126 | 0.366 | 0.763 |
| 56 | 128 | -0.602 | 0.871 |
| 57 | 128 | -0.229 | 0.720 |
| 57 | 130 | -0.561 | 0.716 |
| 57 | 132 | -0.453 | 0.721 |
| 58 | 128 | 0.038 | 0.871 |
| 58 | 130 | -0.410 | 0.867 |
| 58 | 132 | -0.206 | 0.871 |
| 58 | 134 | -0.409 | 0.872 |
| 59 | 128 | 0.433 | 0.719 |
| 59 | 130 | -0.056 | 0.720 |
| 59 | 132 | 0.183 | 0.719 |
| 59 | 134 | -0.074 | 0.719 |
| 59 | 136 | -0.270 | 0.718 |
| 59 | 138 | -0.280 | 0.748 |
| 59 | 140 | -0.256 | 0.807 |
| 59 | 142 | -0.395 | 0.808 |
| 60 | 128 | 0.745 | 0.868 |
| 60 | 130 | 0.143 | 0.871 |
| 60 | 132 | 0.430 | 0.872 |
| 60 | 134 | 0.156 | 0.869 |
| 60 | 136 | 0.014 | 0.868 |
| 60 | 138 | 0.107 | 0.871 |
| 60 | 140 | 0.124 | 0.922 |
| 60 | 142 | 0.017 | 0.996 |
| 60 | 144 | -0.232 | 0.995 |
| 60 | 146 | -0.589 | 0.992 |
| 61 | 130 | 0.582 | 0.720 |
| 61 | 134 | 0.527 | 0.717 |
| 61 | 136 | 0.433 | 0.719 |
| 61 | 138 | 0.592 | 0.718 |
| 61 | 140 | 0.610 | 0.751 |
| 61 | 142 | 0.456 | 0.749 |
| 61 | 144 | 0.176 | 0.748 |
| 61 | 146 | -0.174 | 0.808 |
| 61 | 148 | -0.561 | 0.810 |
| 62 | 144 | 0.555 | 0.923 |
| 62 | 146 | 0.098 | 0.920 |
| 62 | 148 | -0.269 | 0.997 |
| 62 | 150 | -0.543 | 0.992 |
| 63 | 146 | 0.510 | 0.719 |
| 63 | 148 | 0.063 | 0.719 |
| 63 | 150 | -0.149 | 0.806 |
| 63 | 152 | -0.363 | 0.806 |
| 63 | 154 | -0.594 | 0.806 |
| 64 | 148 | 0.391 | 0.869 |
| 64 | 150 | 0.012 | 0.871 |
| 64 | 152 | -0.101 | 0.928 |
| 64 | 154 | -0.347 | 0.925 |
| 65 | 150 | 0.464 | 0.721 |
| 65 | 152 | 0.164 | 0.720 |
| 65 | 154 | 0.080 | 0.765 |
| 65 | 156 | -0.310 | 0.764 |
| 66 | 152 | 0.535 | 0.869 |
| 66 | 154 | 0.243 | 0.871 |
| 66 | 156 | 0.065 | 0.926 |
| 66 | 158 | -0.362 | 0.926 |
| 67 | 154 | 0.627 | 0.719 |
| 67 | 156 | 0.288 | 0.721 |
| 67 | 158 | 0.034 | 0.766 |
| 67 | 160 | -0.308 | 0.765 |
| 68 | 156 | 0.681 | 0.871 |
| 68 | 158 | 0.242 | 0.870 |
| 68 | 160 | -0.048 | 0.926 |
| 68 | 162 | -0.438 | 0.926 |
| 68 | 164 | -0.623 | 0.993 |
| 69 | 160 | 0.244 | 0.720 |
| 69 | 162 | -0.062 | 0.764 |
| 69 | 164 | -0.285 | 0.804 |
| 69 | 166 | -0.440 | 0.805 |
| 69 | 182 | -0.519 | 0.809 |
| 70 | 160 | 0.618 | 0.869 |
| 70 | 162 | 0.191 | 0.871 |
| 70 | 164 | -0.145 | 0.872 |
| 70 | 166 | -0.233 | 0.992 |
| 70 | 168 | -0.351 | 0.992 |
| 70 | 170 | -0.569 | 0.999 |
| 70 | 172 | -0.639 | 0.995 |
| 70 | 182 | -0.199 | 0.994 |
| 70 | 184 | -0.752 | 0.995 |
| 71 | 164 | 0.268 | 0.718 |
| 71 | 166 | -0.045 | 0.718 |
| 71 | 168 | -0.060 | 0.766 |
| 71 | 170 | -0.308 | 0.762 |
| 71 | 172 | -0.287 | 0.805 |
| 71 | 174 | -0.417 | 0.809 |
| 71 | 176 | -0.374 | 0.809 |
| 71 | 178 | -0.447 | 0.810 |
| 71 | 180 | -0.439 | 0.808 |
| 71 | 182 | 0.120 | 0.806 |
| 71 | 184 | -0.395 | 0.808 |
| 72 | 164 | 0.582 | 0.870 |
| 72 | 166 | 0.333 | 0.869 |
| 72 | 168 | 0.117 | 0.870 |
| 72 | 170 | -0.058 | 0.927 |
| 72 | 172 | -0.018 | 0.928 |
| 72 | 174 | -0.184 | 0.993 |
| 72 | 176 | -0.016 | 0.994 |
| 72 | 178 | -0.126 | 0.995 |
| 72 | 180 | -0.158 | 0.998 |
| 72 | 182 | 0.426 | 0.994 |
| 72 | 184 | -0.142 | 0.994 |
| 73 | 168 | 0.562 | 0.720 |
| 73 | 170 | 0.214 | 0.720 |
| 73 | 172 | 0.376 | 0.765 |
| 73 | 174 | 0.174 | 0.765 |
| 73 | 176 | 0.277 | 0.766 |
| 73 | 178 | 0.256 | 0.809 |
| 73 | 180 | 0.166 | 0.808 |
| 73 | 184 | 0.219 | 0.809 |
| 74 | 170 | 0.627 | 0.871 |
| 74 | 172 | 0.555 | 0.869 |
| 74 | 174 | 0.490 | 0.926 |
| 74 | 176 | 0.588 | 0.924 |
| 74 | 178 | 0.582 | 0.993 |
| 74 | 180 | 0.495 | 0.992 |
| 74 | 184 | 0.475 | 0.998 |
| 82 | 186 | -0.603 | 0.869 |
| 83 | 186 | -0.301 | 0.719 |
| 84 | 186 | -0.086 | 0.873 |
| 85 | 186 | 0.229 | 0.718 |
| 85 | 188 | -0.523 | 0.718 |
| 85 | 190 | -0.499 | 0.719 |
| 85 | 198 | -0.611 | 0.807 |
| 86 | 186 | 0.459 | 0.870 |
| 86 | 188 | -0.283 | 0.868 |
| 86 | 190 | -0.270 | 0.872 |
| 86 | 192 | -0.226 | 0.871 |
| 86 | 194 | -0.235 | 0.870 |
| 86 | 196 | -0.227 | 0.872 |
| 86 | 198 | -0.244 | 0.922 |
| 86 | 200 | -0.270 | 0.921 |
| 86 | 202 | -0.276 | 0.995 |
| 86 | 204 | -0.435 | 0.991 |
| 86 | 206 | -0.610 | 0.993 |
| 87 | 188 | 0.030 | 0.718 |
| 87 | 190 | 0.094 | 0.719 |
| 87 | 192 | 0.137 | 0.720 |
| 87 | 194 | 0.216 | 0.720 |
| 87 | 196 | 0.261 | 0.720 |
| 87 | 198 | 0.231 | 0.750 |
| 87 | 200 | 0.183 | 0.749 |
| 87 | 202 | 0.078 | 0.751 |
| 87 | 204 | -0.048 | 0.805 |
| 87 | 206 | -0.265 | 0.810 |
| 87 | 208 | -0.452 | 0.807 |
| 88 | 188 | 0.276 | 0.870 |
| 88 | 190 | 0.380 | 0.873 |
| 88 | 192 | 0.412 | 0.870 |
| 88 | 194 | 0.569 | 0.871 |
| 88 | 196 | 0.640 | 0.867 |
| 88 | 198 | 0.641 | 0.871 |
| 88 | 200 | 0.556 | 0.921 |
| 88 | 202 | 0.423 | 0.920 |
| 88 | 204 | 0.184 | 0.920 |
| 88 | 206 | -0.004 | 0.992 |
| 88 | 208 | -0.222 | 0.994 |
| 88 | 210 | -0.414 | 0.995 |
| 88 | 212 | -0.610 | 0.993 |
| 89 | 204 | 0.543 | 0.751 |
| 89 | 206 | 0.280 | 0.752 |
| 89 | 208 | 0.096 | 0.807 |
| 89 | 210 | -0.111 | 0.806 |
| 89 | 212 | -0.313 | 0.808 |
| 89 | 214 | -0.496 | 0.807 |
| 90 | 206 | 0.573 | 0.873 |
| 90 | 208 | 0.264 | 0.870 |
| 90 | 210 | 0.123 | 0.924 |
| 90 | 212 | -0.132 | 0.924 |
| 90 | 214 | -0.327 | 0.927 |
| 90 | 216 | -0.490 | 0.993 |
| 90 | 218 | -0.707 | 0.992 |
| 91 | 210 | 0.359 | 0.720 |
| 91 | 212 | 0.157 | 0.768 |
| 91 | 214 | -0.002 | 0.764 |
| 91 | 216 | -0.248 | 0.764 |
| 91 | 218 | -0.461 | 0.808 |
| 92 | 210 | 0.621 | 0.869 |
| 92 | 212 | 0.293 | 0.871 |
| 92 | 214 | 0.155 | 0.928 |
| 92 | 216 | -0.019 | 0.929 |
| 92 | 218 | -0.311 | 0.927 |
| 92 | 220 | -0.491 | 0.992 |
| 92 | 222 | -0.668 | 0.998 |
| 93 | 212 | 0.628 | 0.719 |
| 93 | 214 | 0.388 | 0.721 |
| 93 | 216 | 0.225 | 0.764 |
| 93 | 218 | -0.034 | 0.765 |
| 93 | 220 | -0.312 | 0.765 |
| 93 | 222 | -0.498 | 0.764 |
| 93 | 252 | -0.782 | 0.811 |
| 93 | 254 | -0.742 | 0.814 |
| 93 | 256 | -0.835 | 0.813 |
| 94 | 214 | 0.628 | 0.867 |
| 94 | 216 | 0.376 | 0.870 |
| 94 | 218 | 0.111 | 0.871 |
| 94 | 220 | -0.161 | 0.927 |
| 94 | 222 | -0.367 | 0.927 |
| 94 | 224 | -0.573 | 0.926 |
| 94 | 252 | -0.735 | 1.000 |
| 94 | 254 | -0.654 | 0.998 |
| 94 | 256 | -0.704 | 0.999 |
| 95 | 218 | 0.393 | 0.719 |
| 95 | 220 | 0.125 | 0.718 |
| 95 | 222 | -0.122 | 0.764 |
| 95 | 224 | -0.271 | 0.766 |
| 95 | 226 | -0.419 | 0.763 |
| 95 | 252 | -0.701 | 0.812 |
| 95 | 254 | -0.521 | 0.814 |
| 95 | 256 | -0.480 | 0.813 |
| 96 | 220 | 0.303 | 0.871 |
| 96 | 222 | -0.002 | 0.871 |
| 96 | 224 | -0.090 | 0.927 |
| 96 | 226 | -0.302 | 0.927 |
| 96 | 228 | -0.417 | 0.926 |
| 96 | 230 | -0.520 | 0.927 |
| 96 | 232 | -0.579 | 0.992 |
| 96 | 234 | -0.745 | 0.995 |
| 96 | 252 | -0.749 | 1.002 |
| 96 | 254 | -0.485 | 0.999 |
| 96 | 256 | -0.359 | 0.996 |
| 97 | 222 | 0.283 | 0.722 |
| 97 | 224 | 0.068 | 0.719 |
| 97 | 226 | 0.013 | 0.763 |
| 97 | 228 | -0.155 | 0.765 |
| 97 | 230 | -0.300 | 0.765 |
| 97 | 232 | -0.365 | 0.807 |
| 97 | 234 | -0.532 | 0.806 |
| 97 | 240 | -0.662 | 0.808 |
| 97 | 242 | -0.589 | 0.815 |
| 97 | 244 | -0.616 | 0.814 |
| 97 | 252 | -0.667 | 0.815 |
| 97 | 254 | -0.395 | 0.811 |
| 97 | 256 | -0.181 | 0.814 |
| 98 | 222 | 0.511 | 0.869 |
| 98 | 224 | 0.281 | 0.870 |
| 98 | 226 | 0.122 | 0.873 |
| 98 | 228 | 0.027 | 0.927 |
| 98 | 230 | -0.151 | 0.925 |
| 98 | 232 | -0.276 | 0.929 |
| 98 | 234 | -0.418 | 0.993 |
| 98 | 236 | -0.585 | 0.996 |
| 98 | 238 | -0.638 | 0.993 |
| 98 | 240 | -0.529 | 0.996 |
| 98 | 242 | -0.433 | 0.995 |

**$S_{2n}$ (even N)**

| Z | N | $S_{2n}$ | $\sigma_{S_{2n}}$ |
|---|---|---|---|
| 98 | 244 | -0.527 | 0.994 |
| 98 | 246 | -0.610 | 0.994 |
| 98 | 248 | -0.642 | 0.991 |
| 98 | 250 | -0.674 | 0.994 |
| 98 | 252 | -0.640 | 0.994 |
| 98 | 254 | -0.368 | 0.994 |
| 98 | 256 | -0.103 | 1.001 |
| 99 | 224 | 0.622 | 0.718 |
| 99 | 226 | 0.366 | 0.720 |
| 99 | 228 | 0.238 | 0.720 |
| 99 | 230 | 0.120 | 0.765 |
| 99 | 232 | -0.077 | 0.764 |
| 99 | 234 | -0.214 | 0.805 |
| 99 | 236 | -0.371 | 0.806 |
| 99 | 238 | -0.454 | 0.809 |
| 99 | 240 | -0.323 | 0.810 |
| 99 | 242 | -0.221 | 0.808 |
| 99 | 244 | -0.309 | 0.809 |
| 99 | 246 | -0.447 | 0.808 |
| 99 | 248 | -0.476 | 0.806 |
| 99 | 250 | -0.518 | 0.805 |
| 99 | 252 | -0.516 | 0.809 |
| 99 | 254 | -0.302 | 0.813 |
| 99 | 256 | 0.067 | 0.810 |
| 99 | 258 | -0.782 | 0.809 |
| 100 | 226 | 0.641 | 0.871 |
| 100 | 228 | 0.415 | 0.869 |
| 100 | 230 | 0.243 | 0.871 |
| 100 | 232 | 0.045 | 0.928 |
| 100 | 234 | -0.122 | 0.928 |
| 100 | 236 | -0.248 | 0.993 |
| 100 | 238 | -0.347 | 0.993 |
| 100 | 240 | -0.158 | 0.992 |
| 100 | 242 | -0.079 | 0.994 |
| 100 | 244 | -0.177 | 0.991 |
| 100 | 246 | -0.312 | 0.989 |
| 100 | 248 | -0.382 | 0.990 |
| 100 | 250 | -0.432 | 0.997 |
| 100 | 252 | -0.452 | 0.993 |
| 100 | 254 | -0.297 | 0.993 |
| 100 | 256 | 0.195 | 0.995 |
| 100 | 258 | -0.610 | 0.992 |
| 101 | 230 | 0.453 | 0.718 |
| 101 | 232 | 0.196 | 0.719 |
| 101 | 234 | 0.062 | 0.763 |
| 101 | 236 | -0.068 | 0.764 |
| 101 | 238 | -0.188 | 0.761 |
| 101 | 240 | -0.075 | 0.764 |
| 101 | 242 | 0.173 | 0.807 |
| 101 | 244 | 0.060 | 0.810 |
| 101 | 246 | -0.059 | 0.809 |
| 101 | 248 | -0.160 | 0.805 |
| 101 | 250 | -0.207 | 0.807 |
| 101 | 252 | -0.254 | 0.808 |
| 101 | 254 | -0.184 | 0.808 |
| 101 | 256 | 0.385 | 0.804 |
| 101 | 258 | -0.398 | 0.805 |
| 102 | 230 | 0.624 | 0.874 |
| 102 | 232 | 0.390 | 0.871 |
| 102 | 234 | 0.089 | 0.870 |
| 102 | 236 | 0.019 | 0.872 |
| 102 | 238 | -0.059 | 0.926 |
| 102 | 240 | -0.030 | 0.927 |
| 102 | 242 | 0.293 | 0.927 |
| 102 | 244 | 0.177 | 0.994 |
| 102 | 246 | 0.028 | 0.991 |
| 102 | 248 | -0.070 | 0.994 |
| 102 | 250 | -0.120 | 0.995 |
| 102 | 252 | -0.174 | 0.994 |
| 102 | 254 | -0.143 | 0.991 |
| 102 | 256 | 0.422 | 0.996 |
| 102 | 258 | -0.282 | 0.992 |
| 103 | 234 | 0.327 | 0.719 |
| 103 | 236 | 0.132 | 0.718 |
| 103 | 238 | 0.169 | 0.764 |
| 103 | 240 | 0.130 | 0.763 |
| 103 | 242 | 0.490 | 0.765 |
| 103 | 244 | 0.438 | 0.766 |
| 103 | 246 | 0.303 | 0.808 |
| 103 | 248 | 0.182 | 0.806 |
| 103 | 250 | 0.112 | 0.806 |
| 103 | 252 | 0.017 | 0.809 |
| 103 | 254 | 0.018 | 0.809 |
| 103 | 256 | 0.605 | 0.806 |
| 103 | 258 | -0.075 | 0.807 |
| 104 | 234 | 0.502 | 0.868 |
| 104 | 236 | 0.351 | 0.931 |
| 104 | 238 | 0.292 | 0.926 |
| 104 | 240 | 0.207 | 0.925 |
| 104 | 242 | 0.563 | 0.928 |
| 104 | 244 | 0.625 | 0.924 |
| 104 | 246 | 0.421 | 0.993 |
| 104 | 248 | 0.277 | 0.990 |
| 104 | 250 | 0.208 | 0.993 |
| 104 | 252 | 0.119 | 0.991 |
| 104 | 254 | 0.064 | 0.991 |
| 104 | 256 | 0.662 | 0.993 |
| 104 | 258 | 0.045 | 0.992 |
| 105 | 236 | 0.579 | 0.762 |
| 105 | 238 | 0.516 | 0.762 |
| 105 | 240 | 0.465 | 0.763 |
| 105 | 242 | 0.642 | 0.766 |
| 105 | 246 | 0.634 | 0.764 |
| 105 | 248 | 0.254 | 0.764 |
| 105 | 250 | 0.550 | 0.807 |
| 105 | 252 | 0.271 | 0.807 |
| 105 | 254 | 0.250 | 0.810 |
| 105 | 256 | 0.842 | 0.809 |
| 105 | 258 | 0.245 | 0.809 |
| 106 | 238 | 0.608 | 0.926 |
| 106 | 240 | 0.613 | 0.928 |
| 106 | 242 | 0.667 | 0.928 |
| 106 | 246 | 0.751 | 0.927 |
| 106 | 248 | 0.378 | 0.927 |
| 106 | 250 | 0.780 | 0.995 |
| 106 | 252 | 0.307 | 0.994 |
| 106 | 254 | 0.314 | 0.993 |
| 106 | 256 | 0.941 | 0.996 |
| 106 | 258 | 0.334 | 0.993 |
| 107 | 248 | 0.725 | 0.765 |
| 107 | 252 | 0.638 | 0.764 |
| 107 | 254 | 0.561 | 0.810 |
| 107 | 258 | 0.495 | 0.807 |
| 108 | 250 | 0.799 | 0.926 |
| 108 | 252 | 0.847 | 0.926 |
| 108 | 254 | 0.697 | 0.993 |
| 108 | 258 | 0.538 | 0.994 |
| 108 | 270 | -0.678 | 0.993 |
| 109 | 254 | 0.970 | 0.808 |
| 109 | 258 | 0.780 | 0.807 |
| 109 | 270 | -0.384 | 0.806 |
| 110 | 258 | 0.950 | 0.993 |
| 110 | 260 | -0.898 | 0.996 |
| 110 | 270 | -0.165 | 0.992 |
| 110 | 274 | -0.522 | 0.992 |
| 111 | 260 | -0.666 | 0.809 |
| 111 | 270 | -0.305 | 0.808 |
| 111 | 274 | 0.067 | 0.807 |
| 111 | 276 | -0.872 | 0.806 |
| 111 | 278 | -0.709 | 0.806 |
| 112 | 260 | -0.494 | 0.991 |
| 112 | 270 | -0.529 | 0.994 |
| 112 | 272 | -0.567 | 0.993 |
| 112 | 274 | 0.546 | 0.992 |
| 112 | 276 | -0.405 | 0.994 |
| 112 | 278 | -0.658 | 0.992 |
| 112 | 282 | -0.787 | 0.991 |
| 113 | 260 | -0.266 | 0.809 |
| 113 | 270 | -0.403 | 0.808 |
| 113 | 272 | -0.355 | 0.808 |
| 113 | 274 | 0.383 | 0.809 |
| 113 | 276 | 0.031 | 0.806 |
| 113 | 278 | -0.345 | 0.808 |
| 113 | 280 | -0.870 | 0.808 |
| 113 | 284 | -0.723 | 0.805 |
| 114 | 260 | -0.082 | 0.990 |
| 114 | 266 | -0.800 | 0.992 |
| 114 | 268 | -0.645 | 0.995 |
| 114 | 270 | -0.367 | 0.991 |
| 114 | 272 | -0.252 | 0.996 |
| 114 | 274 | 0.097 | 0.996 |
| 114 | 276 | 0.362 | 0.997 |
| 114 | 278 | -0.127 | 0.994 |
| 114 | 280 | -0.507 | 0.995 |
| 114 | 282 | -0.868 | 0.991 |
| 114 | 284 | -0.690 | 0.994 |
| 114 | 286 | -0.699 | 0.992 |
| 115 | 260 | 0.161 | 0.807 |
| 115 | 262 | -0.692 | 0.811 |
| 115 | 264 | -0.770 | 0.805 |
| 115 | 266 | -0.608 | 0.805 |
| 115 | 268 | -0.418 | 0.807 |
| 115 | 270 | -0.159 | 0.809 |
| 115 | 272 | -0.058 | 0.809 |
| 115 | 274 | 0.501 | 0.809 |
| 115 | 276 | 0.296 | 0.807 |
| 115 | 278 | 0.087 | 0.808 |
| 115 | 280 | -0.415 | 0.809 |
| 115 | 282 | -0.531 | 0.809 |
| 115 | 284 | -0.504 | 0.808 |
| 115 | 286 | -0.500 | 0.807 |
| 115 | 288 | -0.593 | 0.807 |
| 116 | 260 | 0.360 | 0.994 |
| 116 | 262 | -0.434 | 0.998 |
| 116 | 264 | -0.552 | 0.992 |
| 116 | 266 | -0.465 | 0.992 |
| 116 | 268 | -0.291 | 0.994 |
| 116 | 270 | -0.060 | 0.995 |
| 116 | 272 | 0.026 | 0.992 |
| 116 | 274 | 0.760 | 0.992 |
| 116 | 276 | 0.113 | 0.998 |
| 116 | 278 | 0.224 | 0.993 |
| 116 | 280 | -0.416 | 0.995 |
| 116 | 282 | -0.283 | 0.997 |
| 116 | 284 | -0.427 | 0.993 |
| 116 | 286 | -0.412 | 0.990 |
| 116 | 288 | -0.513 | 0.992 |
| 116 | 290 | -0.674 | 0.993 |
| 117 | 262 | -0.218 | 0.809 |
| 117 | 264 | -0.328 | 0.810 |
| 117 | 266 | -0.256 | 0.806 |
| 117 | 268 | -0.040 | 0.807 |
| 117 | 270 | 0.132 | 0.811 |
| 117 | 272 | 0.410 | 0.809 |
| 117 | 274 | 0.827 | 0.809 |
| 117 | 276 | 0.307 | 0.809 |
| 117 | 278 | 0.332 | 0.809 |
| 117 | 280 | 0.065 | 0.806 |
| 117 | 282 | -0.184 | 0.806 |
| 117 | 284 | -0.198 | 0.809 |
| 117 | 286 | -0.242 | 0.805 |
| 117 | 288 | -0.356 | 0.806 |
| 117 | 290 | -0.446 | 0.806 |
| 117 | 292 | -0.567 | 0.806 |
| 118 | 262 | 0.047 | 0.994 |
| 118 | 264 | -0.082 | 0.993 |
| 118 | 266 | -0.076 | 0.993 |
| 118 | 268 | 0.121 | 0.992 |
| 118 | 270 | 0.209 | 0.992 |
| 118 | 272 | 0.656 | 0.993 |
| 118 | 274 | 0.747 | 0.995 |
| 118 | 276 | 0.362 | 0.994 |
| 118 | 278 | 0.352 | 0.990 |
| 118 | 280 | 0.451 | 0.997 |
| 118 | 282 | -0.181 | 0.995 |
| 118 | 284 | -0.062 | 0.995 |
| 118 | 286 | -0.180 | 0.997 |
| 118 | 288 | -0.302 | 0.994 |
| 118 | 290 | -0.339 | 0.991 |
| 118 | 292 | -0.465 | 0.996 |
| 118 | 294 | -0.642 | 0.993 |
| 119 | 262 | 0.265 | 0.807 |
| 119 | 264 | 0.130 | 0.809 |
| 119 | 266 | 0.163 | 0.807 |
| 119 | 268 | 0.374 | 0.805 |
| 119 | 270 | 0.440 | 0.808 |
| 119 | 274 | 0.960 | 0.808 |
| 119 | 276 | 0.744 | 0.811 |
| 119 | 278 | 0.726 | 0.807 |
| 119 | 280 | 0.590 | 0.804 |
| 119 | 282 | 0.154 | 0.807 |
| 119 | 284 | 0.067 | 0.806 |
| 119 | 286 | 0.038 | 0.806 |
| 119 | 288 | -0.096 | 0.807 |
| 119 | 290 | -0.164 | 0.806 |
| 119 | 292 | -0.255 | 0.806 |
| 119 | 294 | -0.402 | 0.807 |
| 119 | 296 | -0.582 | 0.809 |

**$S_{1p}$ (odd Z)**

| Z | N | $S_{1p}$ | $\sigma_{S_{1p}}$ |
|---|---|---|---|
| 25 | 21 | -0.056 | 0.452 |
| 35 | 34 | 0.202 | 0.533 |
| 37 | 36 | 0.237 | 0.573 |
| 39 | 37 | -0.110 | 1.142 |
| 39 | 38 | 0.057 | 0.855 |
| 41 | 39 | -0.554 | 0.783 |
| 41 | 40 | -0.309 | 0.655 |
| 45 | 44 | -0.343 | 0.699 |
| 47 | 46 | -0.377 | 0.713 |
| 49 | 48 | -0.317 | 0.587 |
| 55 | 59 | -0.200 | 0.482 |
| 55 | 60 | -0.017 | 0.445 |
| 57 | 61 | 0.037 | 0.535 |
| 57 | 62 | 0.270 | 0.559 |
| 59 | 63 | -0.141 | 0.534 |
| 59 | 64 | -0.076 | 0.546 |
| 61 | 67 | -0.024 | 0.508 |
| 61 | 68 | 0.127 | 0.536 |
| 63 | 69 | -0.293 | 0.523 |
| 63 | 70 | -0.279 | 0.551 |
| 63 | 71 | 0.261 | 0.501 |
| 63 | 72 | 0.268 | 0.496 |
| 65 | 73 | -0.337 | 0.604 |
| 65 | 74 | -0.222 | 0.521 |
| 67 | 78 | 0.107 | 0.454 |
| 69 | 80 | -0.297 | 0.476 |
| 69 | 81 | 0.168 | 0.410 |
| 71 | 83 | 0.035 | 0.389 |
| 71 | 84 | -0.028 | 0.449 |
| 73 | 85 | -0.189 | 0.371 |
| 73 | 86 | -0.208 | 0.451 |
| 75 | 89 | -0.151 | 0.386 |
| 75 | 90 | 0.021 | 0.545 |
| 77 | 91 | -0.292 | 0.499 |
| 77 | 92 | -0.275 | 0.548 |
| 77 | 93 | 0.101 | 0.380 |
| 77 | 94 | 0.004 | 0.448 |
| 79 | 95 | -0.130 | 0.375 |
| 79 | 96 | -0.351 | 0.614 |
| 79 | 98 | -0.050 | 0.464 |
| 81 | 99 | -0.406 | 0.612 |
| 81 | 100 | -0.196 | 0.468 |
| 81 | 101 | -0.096 | 0.424 |
| 83 | 105 | -0.253 | 0.468 |
| 83 | 106 | -0.271 | 0.544 |
| 85 | 107 | -0.136 | 0.405 |
| 85 | 110 | -0.148 | 0.454 |
| 87 | 113 | -0.215 | 0.373 |
| 87 | 114 | -0.176 | 0.465 |
| 89 | 117 | -0.109 | 0.377 |
| 89 | 118 | -0.146 | 0.450 |
| 91 | 121 | -0.239 | 0.502 |
| 91 | 122 | -0.210 | 0.453 |
| 91 | 123 | 0.104 | 0.388 |
| 93 | 126 | -0.296 | 0.587 |
| 93 | 127 | 0.177 | 0.539 |
| 93 | 128 | 0.229 | 0.595 |
| 95 | 129 | -0.101 | 0.590 |
| 95 | 130 | 0.065 | 0.628 |
| 97 | 131 | 0.043 | 0.629 |
| 97 | 132 | 0.126 | 0.661 |
| 99 | 133 | -0.372 | 0.616 |
| 99 | 134 | -0.277 | 0.568 |
| 99 | 135 | -0.004 | 0.607 |
| 99 | 136 | 0.110 | 0.563 |
| 101 | 137 | -0.258 | 0.535 |
| 101 | 138 | -0.243 | 0.579 |
| 101 | 139 | 0.166 | 0.554 |
| 101 | 140 | 0.149 | 0.557 |
| 103 | 141 | -0.207 | 0.564 |
| 103 | 142 | -0.205 | 0.579 |
| 103 | 143 | 0.156 | 0.551 |
| 103 | 144 | 0.166 | 0.552 |
| 105 | 145 | -0.351 | 0.547 |
| 105 | 146 | -0.304 | 0.552 |
| 105 | 147 | 0.142 | 0.542 |
| 105 | 148 | 0.144 | 0.549 |
| 107 | 149 | -0.236 | 0.564 |
| 107 | 150 | -0.278 | 0.560 |
| 107 | 151 | 0.188 | 0.549 |
| 107 | 152 | 0.190 | 0.556 |
| 109 | 155 | -0.095 | 0.548 |
| 109 | 156 | -0.040 | 0.576 |
| 111 | 159 | -0.044 | 0.534 |
| 111 | 160 | -0.045 | 0.551 |
| 113 | 161 | -0.295 | 0.594 |
| 113 | 162 | -0.313 | 0.608 |
| 113 | 163 | 0.208 | 0.602 |
| 113 | 164 | 0.217 | 0.606 |
| 115 | 165 | -0.107 | 0.578 |
| 115 | 166 | -0.148 | 0.592 |
| 115 | 167 | 0.335 | 0.585 |
| 115 | 168 | 0.316 | 0.576 |
| 117 | 169 | -0.241 | 0.553 |
| 117 | 170 | -0.180 | 0.600 |
| 117 | 171 | 0.302 | 0.599 |
| 117 | 172 | 0.302 | 0.605 |
| 119 | 173 | -0.051 | 0.590 |
| 119 | 174 | -0.111 | 0.587 |
| 119 | 175 | 0.338 | 0.600 |
| 119 | 176 | 0.262 | 0.615 |

**$S_{2p}$ (even Z)**

| Z | N | $S_{2p}$ | $\sigma_{S_{2p}}$ |
|---|---|---|---|
| 14 | 8 | -0.714 | 1.527 |
| 16 | 10 | -0.305 | 1.272 |
| 20 | 14 | -0.679 | 1.334 |
| 24 | 18 | -0.516 | 0.932 |
| 26 | 20 | 0.512 | 0.995 |
| 28 | 22 | 0.598 | 1.201 |
| 30 | 25 | 0.066 | 1.105 |
| 32 | 28 | 0.403 | 1.088 |
| 34 | 30 | 0.365 | 1.015 |
| 36 | 32 | 0.126 | 0.962 |
| 38 | 34 | -0.125 | 1.032 |
| 40 | 36 | -0.004 | 1.162 |
| 42 | 38 | -0.370 | 1.125 |
| 42 | 39 | 0.502 | 1.136 |
| 44 | 40 | -0.822 | 1.256 |
| 44 | 41 | 0.475 | 0.910 |
| 46 | 42 | -0.640 | 1.212 |
| 46 | 43 | 0.440 | 1.062 |
| 48 | 44 | -0.571 | 1.219 |
| 48 | 45 | 0.351 | 1.098 |
| 50 | 47 | 0.175 | 1.175 |
| 58 | 59 | -0.406 | 0.784 |
| 60 | 62 | 0.240 | 0.857 |
| 62 | 65 | -0.370 | 0.758 |
| 62 | 66 | 0.488 | 0.866 |
| 64 | 68 | -0.071 | 0.839 |
| 66 | 71 | -0.302 | 1.031 |
| 66 | 72 | 0.526 | 1.001 |
| 68 | 74 | -0.004 | 0.829 |
| 70 | 77 | -0.207 | 0.708 |
| 72 | 80 | 0.118 | 0.856 |
| 74 | 82 | -0.208 | 0.858 |
| 74 | 83 | 0.318 | 0.727 |
| 76 | 85 | -0.269 | 0.729 |
| 76 | 86 | 0.202 | 0.743 |
| 78 | 89 | -0.420 | 0.700 |
| 82 | 96 | -0.162 | 0.887 |
| 82 | 97 | 0.110 | 0.616 |
| 84 | 102 | -0.446 | 0.835 |
| 86 | 105 | -0.374 | 0.583 |
| 86 | 106 | 0.080 | 0.745 |
| 88 | 109 | -0.323 | 0.704 |
| 88 | 110 | 0.128 | 0.861 |
| 90 | 113 | -0.345 | 0.718 |
| 90 | 114 | 0.005 | 0.829 |
| 90 | 115 | 0.240 | 0.684 |
| 92 | 118 | -0.055 | 0.840 |
| 92 | 119 | 0.105 | 0.696 |
| 92 | 120 | 0.497 | 0.845 |
| 94 | 122 | -0.238 | 0.881 |
| 94 | 123 | 0.083 | 0.750 |
| 94 | 124 | 0.477 | 0.877 |
| 96 | 126 | -0.236 | 0.928 |
| 96 | 127 | 0.194 | 0.850 |
| 98 | 128 | -0.678 | 0.967 |
| 98 | 129 | -0.151 | 0.795 |
| 98 | 130 | 0.537 | 0.935 |
| 100 | 131 | -0.483 | 0.799 |
| 100 | 132 | -0.087 | 0.882 |
| 100 | 133 | 0.189 | 0.789 |
| 102 | 134 | -0.510 | 0.871 |
| 102 | 135 | -0.410 | 0.722 |
| 102 | 136 | 0.092 | 0.875 |
| 102 | 137 | 0.338 | 0.744 |
| 104 | 140 | -0.064 | 0.836 |
| 104 | 141 | 0.323 | 0.756 |
| 106 | 144 | -0.179 | 0.893 |
| 106 | 145 | 0.065 | 0.750 |
| 108 | 148 | -0.307 | 0.874 |
| 108 | 149 | -0.002 | 0.759 |
| 110 | 152 | -0.570 | 0.886 |
| 110 | 153 | -0.314 | 0.780 |
| 110 | 154 | 0.143 | 0.871 |
| 110 | 155 | 0.473 | 0.788 |
| 112 | 157 | -0.415 | 0.752 |
| 112 | 158 | 0.115 | 0.887 |
| 112 | 159 | 0.443 | 0.740 |
| 114 | 160 | -0.400 | 0.902 |
| 114 | 161 | -0.045 | 0.767 |
| 114 | 162 | 0.461 | 0.930 |
| 116 | 164 | -0.165 | 0.925 |
| 116 | 165 | 0.194 | 0.788 |
| 118 | 169 | -0.116 | 0.815 |
| 118 | 170 | 0.596 | 1.002 |
